# Supplementary material for: Direct digital synthesis of microwave waveforms for quantum computing
Source: arXiv:1703.00942 source file (2017-03-02)
Supplement: Supplementary file 1 [file Supplement.pdf]

# Supplementary material for: Direct digital synthesis of microwave waveforms for quantum computing

March 1, 2017

## 1 Wiring

A wiring diagram of the experiment in the 'full DDS mode' (see Main Text) is shown in Figure. 1. A Keysight M8195a AWG was used in a two-channel, two-marker mode with a maximum sampling rate in this mode of 32 GS/s. In order to guarantee a consistent phase reference for readout, a local oscillator was synthesized on the second channel. The readout pulse was always placed at least 5 $\mu$s after the start of local oscillator generation to ensure a steady-state had been reached. Homodyne detection was performed by mixing down to DC with the local oscillator, low-pass filtering, and aquiring the I and Q quadratures at 1.6 GS/s. The third AWG channel was used as a marker to trigger the Keysight M9703A digitizer housed in the same chassis, which was used for acquisition.

Room temperature amplification and filtering of the input signal was required to ensure pulse amplitudes for the qubit and cavity pulses were comparable during synthesis (see Main Text). Attenuation and filtering were used on the various temperature stages of the dilution refrigerator to minimize environmental noise and maintain high qubit coherence. The 29 GHz low pass filters are Picosecond 5935. The 5.5 GHz pass band filter on the input line (Mini-Circuits VBFZ 5500S+) provides extra attenuation at the cavity frequency. The 26 GHz low pass filters are custom built eccosorb filters. The 4.5 GHz high pass filter (Mini-Circuit VHF 3800+) on the output passes both qubit and cavity tones. The 6.6 GHz high pass filter (Mini-Circuit VHF 5500+) on the output filters out qubit pulses before amplification.

A Travelling Wave Parametric Amplifier (TWPA) was used to amplify the readout signal. A CW tone at 8.2 GHz (generated by a Keysight E8267D PSG Vector Signal Generator) was sent down a separate fridge line and used to pump the TWPA. The TWPA was isolated from the experiment using two circulators (Quinstar QCY-100400XM00). Following the TWPA were two isolators (Quinstar QCI-080800XM00) followed by a high-electron-mobility transistor amplifier (Low Noise Factory LNF-LNC7_10A) and room temperature amplification (MITEQ AFS3-00101200-18-10P-4).

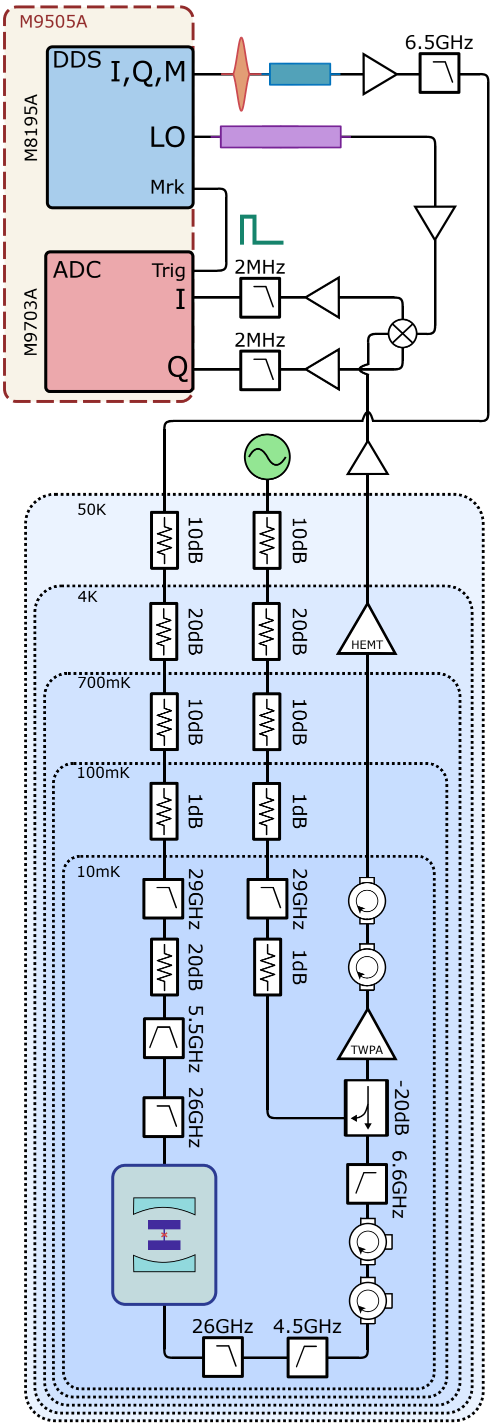


Figure 1: Hardware diagram for the experiment. The Keysight M8195A AWG and M9703A digitizer are both AXIe instrument modules housed in the M9505A Chassis. A single channel of the AWG is sufficient to directly draw both the qubit and readout pulses. A second channel is used to generate the local oscillator used for homodyne detection.

## 2 Phase Noise

The analysis shown here follows Ball et al. [1], and their detailed supplementary information provides an exellent theoretical introduction to clock-induced errors in quantum systems.

Unreliability of a local oscillator (LO) used as a reference clock can lead to effective dephasing of a qubit. LO frequency instability introduces random phase accumulation relative to the qubit (even if the qubit frequency is assumed to be perfectly stable). The unwanted LO phase noise $\phi_N(t)$ can be described as a time dependent frequency detuning $\delta\omega_{LO}(t) = \dot{\phi_N}(t)$, which introduces an LO dephasing term $H_{\phi_N} = \frac{1}{2}\dot{\phi_N}(t)\hat{\sigma_z}$ in the system Hamiltonian [1]. However, when including a non-commuting applied control pulse $U_c$ the $\sigma_z$ operator is rotated due to the control. The LO dephasing term therefore induces both dephasing and damping errors, which can be characterized by a set of filter functions $y_{z,n}(t) = Tr(U_c^\dagger(t)\sigma_z U_c(t)\sigma_n)/2$ for $n \in x, y, z$ [1, 2, 3]. An upper bound of fidelity ($F$) can be found using the measured single sideband phase noise $\hat{\mathcal{L}}(\omega)$ and the filter functions for the control pulse $y_{m,n}(\omega) = -i\omega \int_{-\infty}^{\infty} y_{m,n}(t)e^{i\omega t}$ using [1]

$$F \approx \frac{1}{2}(1 + \exp[-\chi)]) \tag{1}$$

$$\chi = \frac{1}{2\pi}\int_0^\infty d\omega 10^{\frac{\mathcal{L}(\omega)}{10}} \sum_{n\in x,y,z} |y_{z,n}(\omega)|^2 \tag{2}$$

To evaluate the suitability of the DDS system for quantum information applications, we estimate the error introduced by clock instability for two different control operations, an $X_\pi$ gate and an identity gate, and compare the results to an rf source commonly used in quantum experiments (see Main Text). The transfer functions for the $X_\pi$ gate can be calculated using the control propagator (following Green et al. [2])

$$U_c = \exp(-if(t)\sigma_x/2) \tag{3}$$

where $f(t) = \Omega t$ for a square $X_\pi$ pulse or $f(t) = \frac{\sqrt{8\pi}}{\tau}\exp(\frac{-(t-\tau/2)^2}{(2(\tau/4)^2)})$ for a gaussian pulse. $\Omega = \pi/\tau$ is the Rabi rate. The non-zero transfer functions are given by:

$$y_{z,z}(\omega) = -i\omega \int_0^\tau dt\, \cos\big(f(t)\big)e^{i\omega t} \tag{4}$$

$$y_{z,y}(\omega) = -i\omega \int_0^\tau dt\, \sin\big(f(t)\big)e^{i\omega t} \tag{5}$$

For the square pulse this yields

$$y_{z,z}(w) = \frac{\omega^2}{\omega^2 - \Omega^2}(e^{i\omega\tau} + 1) \tag{6}$$

$$y_{z,y}(\omega) = \frac{i\omega\Omega}{\omega^2 - \Omega^2}(e^{i\omega\tau} + 1) \tag{7}$$

The transfer function for the gaussian pulse does not have an analytical form in frequency space, but can be solved numerically.

For free evolution we have a control propagator

$$U_c = \exp(-i\, It/2) \tag{8}$$

and the only nonzero transfer function

$$y_{z,z}(\omega) = 4\sin^2(\omega\tau/2) \tag{9}$$

## References


[1] H. Ball, W. D. Oliver, and M. J. Biercuk. Upper-bounds on qubit coherence set by master clock instabilities. pages 1–13, 2016.

[2] Todd Green, Hermann Uys, and Michael J. Biercuk. High-order noise filtering in nontrivial quantum logic gates. *Physical Review Letters*, 109(2):1–5, 2012.

[3] Todd J. Green, Jarrah Sastrawan, Hermann Uys, and Michael J. Biercuk. Arbitrary quantum control of qubits in the presence of universal noise. *New Journal of Physics*, 15, 2013.
